# Supplementary material for: oLMpics -- On what Language Model Pre-training Captures
Source: arXiv:1912.13283 source file (2020-11-19)
Supplement: Supplementary file 1 [file 08_supp_games.tex]

\clearpage
\newpage
\appendix
\section{Supplementary Experiments}

\subsection{Baseline Tasks}
\label{sec:baseline_tasks}
We first present a few baseline tasks we will build on in later tasks and that aid in understanding the experimental setup and metrics.

%Here we present some baseline tasks to aid in understanding the metrics used, some of which are used later in downstream tasks.

%%%%%%%%%%%%%%%%%%%%%%%%%%%%%%%%%%%%%%%%%%%%%%%%%%%%%%%%%%%%%%%%%%%%%%%%
\paragraph{Multi-choice language modeling}
As a sanity check, we construct a 3-way \multichoicelm{} task. For instance, an example will include the statement \nl{the film was released in the US and [MASK] well at the box office.} and $K=3$ answer candidates: \nl{recurring}, \nl{always} and the gold answer \nl{performed}. 

\noindent
\bfemph{probe construction}

\at{yanai can you please fill this?}

\noindent
\bfemph{results}
Table~\ref{tab:multichoicelm} presents zero-shot accuracy, \smetric{}, and \maxmetric{} for $\MLP{}$ and \linear{}. As expected, all LMs perform very well, close to 100\% accuracy. \mlmbaseline{}, which uses \textsc{GloVe} representations, achieves a maximum of 52\% accuracy (random is 33\%).

We also evaluate this task in the \mcqa{} setup (\S\ref{sec:models}). The Maximum accuracy is comparable to the \mcmlm{} setup, but since the parameters of  $\MLPQA{}$ need to be trained during fine-tuning, the \smetric{} is substantially lower. 
%\at{should we also have results for the ESIM baseline here?}
%\at{show learning curve?} 

\begin{table}[h]
\centering
\resizebox{1.0\columnwidth}{!}{
\begin{tabular}{l|c|cc|cc|cc}
 Model & Zero & \multicolumn{2}{c|}{$\MLP{}$} & \multicolumn{2}{c|}{\linear{}}
 & \multicolumn{2}{c}{\langsenses{}}  \\ 
\toprule
& shot &\smetric{}&\maxmetric{}&\smetric{}&\maxmetric{}&\pertlangs{}& \nolangs{}\\
\midrule
RoBERTa-L &  96 &  96 &  97 &  96 &  97 &   72 &  95 \\
BERT-WWM  &  98 &  98 &  99 &  98 &  98 &   86 &  98 \\
BERT-L    &  98 &  98 &  98 &  92 &  98 &   77 &  95 \\
\hdashline
BERT-B    &  98 &  98 &  98 &  98 &  98 &   78 &  96  \\
RoBERTa-B &  95 &  95 &  96 &  95 &  95 &   80 &  94 \\
\hdashline
Baseline  &  47 &  38 &  52 &   - &  -  &   - &   - \\
\end{tabular}}
\caption{\multichoicelm{}.  \at{for the MC-QA perhaps we should have a column separator in bold?} \jb{yes}} 
\label{tab:multichoicelm}
\end{table}

%%%%%%%%%%%%%%%%%%%%%%%%%%%%%%%%%%%%%%%%%%%%%%%%%%%%%%%%%%%%%%%%%%%%%%

\paragraph{Lexical-semantic knowledge}
\textsc{ConceptNet} \cite{speer2017conceptnet} is a Knowledge-Base (KB) that specifies semantic relations between words and concepts in English, and fine-tuning LMs on the knowledge it contains will be useful in later reasoning tasks.
Following \newcite{Bosselut2019COMETCT}, we show fine-tune LMs to predict \textsc{ConceptNet} facts.

\noindent
\bfemph{Probe Construction}
\textsc{ConceptNet} contains more than 34 million triples of the form (\texttt{subject}, \texttt{predicate}, \texttt{object}). We first construct pseudo-language statements 
by mapping each predicate to a natural language phrase. For example, we map the predicate \texttt{atLocation} to \nl{can usually be found at} to obtain statements like \nl{flower can usually be found at [MASK].}, masking the \texttt{object} concept. We use 15 predicates from \textsc{ConceptNet} and create two distractors by randomly choosing an \texttt{object} that occurs in the context of the example \texttt{predicate}, but with a different \texttt{subject}.

\jb{explain train-dev split}
\at{TODO - examples for this task are show in the task examples table that we will add... }

\noindent
\bfemph{Results}
Table~\ref{tab:lexicalsemnatic} shows the result for this task.
Zero-shot performance is lower than the \smetric{} and \maxmetric{}, implying that the LMs had to adapt to the pseudo-language in the task. \bertwwm{} achieves the highest accuracy of 68\% zero-shot, and a maximum of 80\%.  The \mlmbaseline{} is incapable of solving the task, which requires substantial amounts of lexical-semantic knowledge and achieve a close to random result of 33\% \smetric{}-metric and a maximum of 38\%. \jb{I don't like \smetric{}-metric sounds weird}

\at{I'm actually not sure the \partlang{} control is very interesting here, perhaps remove it from the table? }
\at{i don't think we need a learning curve here ...} \jb{yes to both.}

\begin{table}[h]
\centering
\resizebox{1.0\columnwidth}{!}{
\begin{tabular}{l|c|cc|cc|cc}
 Model & Zero & \multicolumn{2}{c|}{$\MLP{}$} & \multicolumn{2}{c|}{\linear{}}
 & \multicolumn{2}{c}{\langsenses{}}  \\ 
\toprule
& shot &\smetric{}&\maxmetric{}&\smetric{}&\maxmetric{}&\pertlangs{}& \nolangs{}\\ 
\midrule
RoBERTa-L &  56 &  59 &  68 &  57 &  63 &   0 &  24 \\
BERT-WWM  &  68 &  71 &  80 &  68 &  73 &   5 &  17 \\
BERT-L    &  43 &  44 &  47 &  43 &  45 &   3 &   0 \\
\hdashline
BERT-B    &  49 &  54 &  76 &  52 &  72 &   9 &   1 \\
RoBERTa-B &  53 &  57 &  68 &  55 &  62 &   1 &  15 \\
\hdashline
Baseline  &  32 &  33 &  38 &   - &  -  &   0 &   0 \\
\end{tabular}}
\caption{\textsc{Lexical-semantic knowledge}.} 
\label{tab:lexicalsemnatic}
\end{table}

%%%%%%%%%%%%%%%%%%%%%%%%%
\subsection{Can LMs capture the \nl{long-tail} of Encyclopedic knowledge?}
Acquiring knowledge from LMs have received an increasingly amount of attention lately \cite{logan2019barack,petroni2019language,xiong2020pretrained}.
Recent language models all uses Wikipedia as part of their training data and since it contains a lot of encyclopedic knowledge, we are interested in LMs ability to capture this kind of information. Recently, \citet{petroni2019language} \at{cite \url{https://arxiv.org/abs/1911.03681}} showed that Bert, does indeed capture some encyclopedic-knowledge facts, and achieves comparable performances to specialized KB construction systems, especially on the 1-to-1 relations (e.g. \textit{capital of}). In their work, they use multiple data sources, such as triplets from Wikipedia \cite{elsahar2018t}, Google-RE,\footnote{\url{https://code.google.com/archive/p/relation-extraction-corpus/}} ConceptNet \cite{speer2017conceptnet} and Squad \cite{squad2016url}.
We note that some of these facts, are indeed expected to be successfully completed due to very explicit queues from the query (e.g. ``The official language of Lithuania is [MASK].'', which is successfully completed to \textbf{Lithuanian}, or ``Jules de Gaultier was born in the city of [MASK].'' which is succesfully completed to \textbf{Paris}, the largest city in France).
In contrast, in this probe, we aim to inspect the \nl{long-tail} distribution of encyclopedic knowledge.

% cite \cite{logan2019barack} - https://arxiv.org/pdf/1906.07241.pdf.
% cite \cite{xiong2020pretrained} - https://arxiv.org/pdf/1912.09637.pdf.

\bfemph{Probe Construction}
We follow \cite{petroni2019language} and use the Google-RE data triplets in order to query the LMs. We use the three relations from this dataset, specifically \textit{birth-place}, \textit{birth-date} and \textit{death-place}. For constructing distractors for the location relations,\footnote{we only use the city locations as answers} we use cities from the same country, whereas for the date relations,\footnote{which consists of the year when the event happened} the distractors arrive from a random window size of 2 years.
We split the data into train/dev according to the following: countries with less than 8 possible cities, go into training, for the rest, we sort the cities based on their population size such as the smaller cities are used in the dev split, and larger would be used in training. The distractors are drawn from cities with similar population size (from a window size of 2 for each side).

\bfemph{Results}
The results of this experiments are summarized in Table \ref{tab:res-encyclopedic}. We note that the results across models are low, do not improve by training and demonstrate low sensitivity to language, implying that LMs contain some encyclopedic knowledge, but cannot acquire more of it by training on this task.

% \begin{itemize}
% \item cite Sebastian Riedel and show we get the same result \cite{lama}
% \item Show that language model do not capture the long-tail well
% \item say this could be a test-bed for research on combining IR and language modeling ...
% \end{itemize}

\begin{table}[h]
\centering
\resizebox{1.0\columnwidth}{!}{
\begin{tabular}{l|c|cc|cc|cc}
 Model & Zero & \multicolumn{2}{c|}{$\MLP{}$} & \multicolumn{2}{c|}{\linear{}}
 & \multicolumn{2}{c}{\langsenses{}}  \\ 
\toprule
& shot &\smetric{}&\maxmetric{}&\smetric{}&\maxmetric{}&\pertlangs{}& \nolangs{}\\ 
\midrule
RoBERTa-L &  48 &  47 &  49 &  46 &  49 &   0 &   1 \\
BERT-WWM  &  52 &  50 &  54 &  50 &  54 &   1 &   2 \\
BERT-L    &  46 &  46 &  50 &  45 &  49 &   0 &   0 \\
\hdashline
BERT-B    &  48 &  47 &  51 &  46 &  51 &   0 &   1 \\
RoBERTa-B &  48 &  47 &  51 &  47 &  49 &   0 &   2 \\
\hdashline
Baseline  &  33 &  33 &  41 &   - &  - &   0 &   0 \\
\end{tabular}}
\caption{Encyclopedic} 
\label{tab:res-encyclopedic}
\end{table}

\subsection{Can LMs handle ``set-negation"?}
The set of objects that have some property is the complement of the set of objects that do not. We test whether LM can handle this case, building on the \textsc{Lexical-semantic knowledge} probe from \S\ref{sec:baseline_tasks}.

%Building on the lexical-semantic similarity baseline probe presented in (\S\ref{sec:baseline_tasks}), here we test if adding a negation to a ConceptNet relation, changes the LMs behavior.

\noindent
\bfemph{Probe Construction}
Our setup is identical to \textsc{Lexical-semantic knowledge}, where we build statements from \texttt{subject predicate object} triples, except that in 50\% of the examples, we add the word \nl{not}: \nl{[MASK] is \textbf{not} a prerequisite of eating.}. Then we sample two concepts from \textsc{ConceptNet} that have the described property and are the distractors (\nl{food}, \nl{chewing}), and one concept that does not (\nl{ticket}), which is the gold answer.

%To achieve this we introduce the notion of a false edge, by sampling a (\texttt{subject},\texttt{predicate}) from the ConceptNet edges, and randomly choosing an \texttt{object} from concepts that do not share an edge with this \texttt{subject}. 
%We use the same experiment design used in the Lexical-Similarity probe, except here we convert 50\% of the examples phrases to a negation, such as \nl{[MASK] is \textbf{not} a prerequisite of eating  . }. In these negation examples, instead of choosing one correct edge as the gold answer, we choose the false edge \texttt{object} as the correct answer (i.e. \nl{ticket}), and use two correct edge \texttt{object}s as distractors (i.e. \nl{food}, \nl{chewing}). 

\noindent
\bfemph{Results}
Results in the task are slightly above random, which is 33\%.  \bertwwm{} achieves the highest zero-shot accuracy, \smetric{} and \maxmetric{} scores of 47, 47, and 51 respectively. In this setting, fine-tuning only slightly improves performance. Error analysis shows that negation examples account for the majority of errors, and the language controls show that there is very little sensitivity to the words in the input. 
These results are aligned with previous results showing that LMs struggle with negation. 

\begin{table}[h]
\centering
\resizebox{1.0\columnwidth}{!}{
\begin{tabular}{l|c|cc|cc|cc}
 Model & Zero & \multicolumn{2}{c|}{MLP} & \multicolumn{2}{c|}{Linear} 
 & \multicolumn{2}{c}{Language}  \\ 
\toprule
          & Acc   &  S     & Max    & S      & Max    & part   & full   \\ 
\midrule
RoBERTa-L &  38 &  39 &  44 &  39 &  42 &   0 &   0 \\
BERT-WWM  &  47 &  47 &  51 &  47 &  49 &   0 &   1 \\
BERT-L    &  40 &  40 &  42 &  40 &  43 &   0 &   0 \\
\hdashline
BERT-B    &  41 &  41 &  45 &  41 &  43 &   0 &   5 \\
RoBERTa-B &  42 &  42 &  45 &  42 &  45 &   0 &   3 \\
\hdashline
Baseline  &  35 &  34 &  38 &   - &   - &   0 &   0 \\
\end{tabular}}
\caption{\textsc{Negation}.} 
\label{tab:negation}
\end{table}

\at{ should we add to the learning curves the MC-QA version of this experiment? remember it was this sudden jump in performance, could be more interesting, because in the MC-MLM setup the models do not succeed at all ... (at least when not fine-tuned on the lexical semantic similarity used to build the task.  } \jb{if it is more successful you can put it in the table?}
